# Supplementary material for: Residual-augmented flow matching operators for probabilistic partial differential equations
Source: arXiv:2512.12749 source file (2026-09-05)
Supplement: Supplementary file 2 [file additional_results.tex]

\section{Additional results and details}
This section contains additional details and results for the experiments presented in the main manuscript.
For each experiment performed, we require samples from a Gaussian process measure.
In our work, we consider a zero-mean (that is, $m_0=0$) Gaussian process parameterized by a Matern covariance kernel with smoothness factor $\nu=0.5$ and length scale of $10^{-3}$.
We implement this using the $\texttt{GPyTorch}$ library \cite{gardner2018gpytorch}.
To model the vector fields using an operator, we propose a conditional Fourier neural operator~\cite{li2020fourier} leveraging feature-wise linear modulation (FiLM)~\cite{perez2018film}, called FiLMFNO, using the $\texttt{neuraloperator}$ library~\cite{kossaifi2025librarylearningneuraloperators}.
The hyperparameters for FiLMFNO have the same meaning as described in the $\texttt{neuraloperator}$ library.
For all experiments, we have considered $4$ Fourier layers, $64$ hidden channels, $4$ lifting channel ratio, and $4$ projection channel ratio.
To compute the coefficients of the FiLM layers, we use fully connected neural networks with $3$ hidden layers of $64$ neurons each and SiLU activations.
To train the model, we use Adam optimizer with a learning rate of $10^{-3}$ and a weight decay of $10^{-4}$.
We use an exponential learning rate scheduler with a decay rate of $0.99$.
To integrate the vector-fields, we use $\texttt{dopri5}$ provided in $\texttt{torchdiffeq}$~\cite{chen2018neural} with $\texttt{atol}=\texttt{rtol}=10^{-5}$.
All experiments are performed using a single NVIDIA H100 GPU.

%% >>> AP1
\subsection{Artificial Benchmark 1: 1D problem with input function dependent correlation}\label{sec:appendix/onedcorr}
% We have considered two sets of experiments, one where the training and inference resolution is the same ($N_x = 128$), and another where the training resolution is coarser than the inference resolution (training on $N_x = \{8, 16, 32, 64\}$ and inference on $N_x = 128$).
For training the models, the configurations are tabulated in~\cref{tab:onedcorr/config}.
% For both sets of experiments, the configurations are tabulated in~\cref{tab:onedcorr/config}
\begin{table}[h!]
\centering
\caption{Training configurations for the 1D problem with input function correlation.
Both equal-resolution and multi-resolution settings are reported.}
\label{tab:onedcorr/config}
\begin{tabular}{cccccc}
\toprule
\makecell{\textbf{Train$\to$Infer}\\\textbf{Resolution}} &
\textbf{Epochs} &
\makecell{\textbf{Train}\\\textbf{Size}} &
\makecell{\textbf{Validation}\\\textbf{Size}} &
\makecell{\textbf{Batch}\\\textbf{Size}} &
\makecell{\textbf{\# Fourier}\\\textbf{Modes}} \\
\midrule
\multirow{4}{*}{128 $\to$ 128}
    & \multirow{4}{*}{300} & 10      & \multirow{4}{*}{1{,}000} & 2   & \multirow{4}{*}{64} \\
& & 50      &  & 4   & \\
& & 500     & & 16  & \\
& & 1{,}000 & & 64  & \\
\midrule
    $8\to128$ & \multirow{4}{*}{300} & \multirow{4}{*}{10}      & \multirow{4}{*}{1{,}000}& \multirow{4}{*}{2}   & 4 \\
$16\to128$&  & & & & 8\\
$32\to128$& & & & & 16\\
$64\to128$& & & & & 32\\
\bottomrule
\end{tabular}
\end{table}
\begin{figure}[h!]
    \centering
    \includegraphics[width=0.8\textwidth]{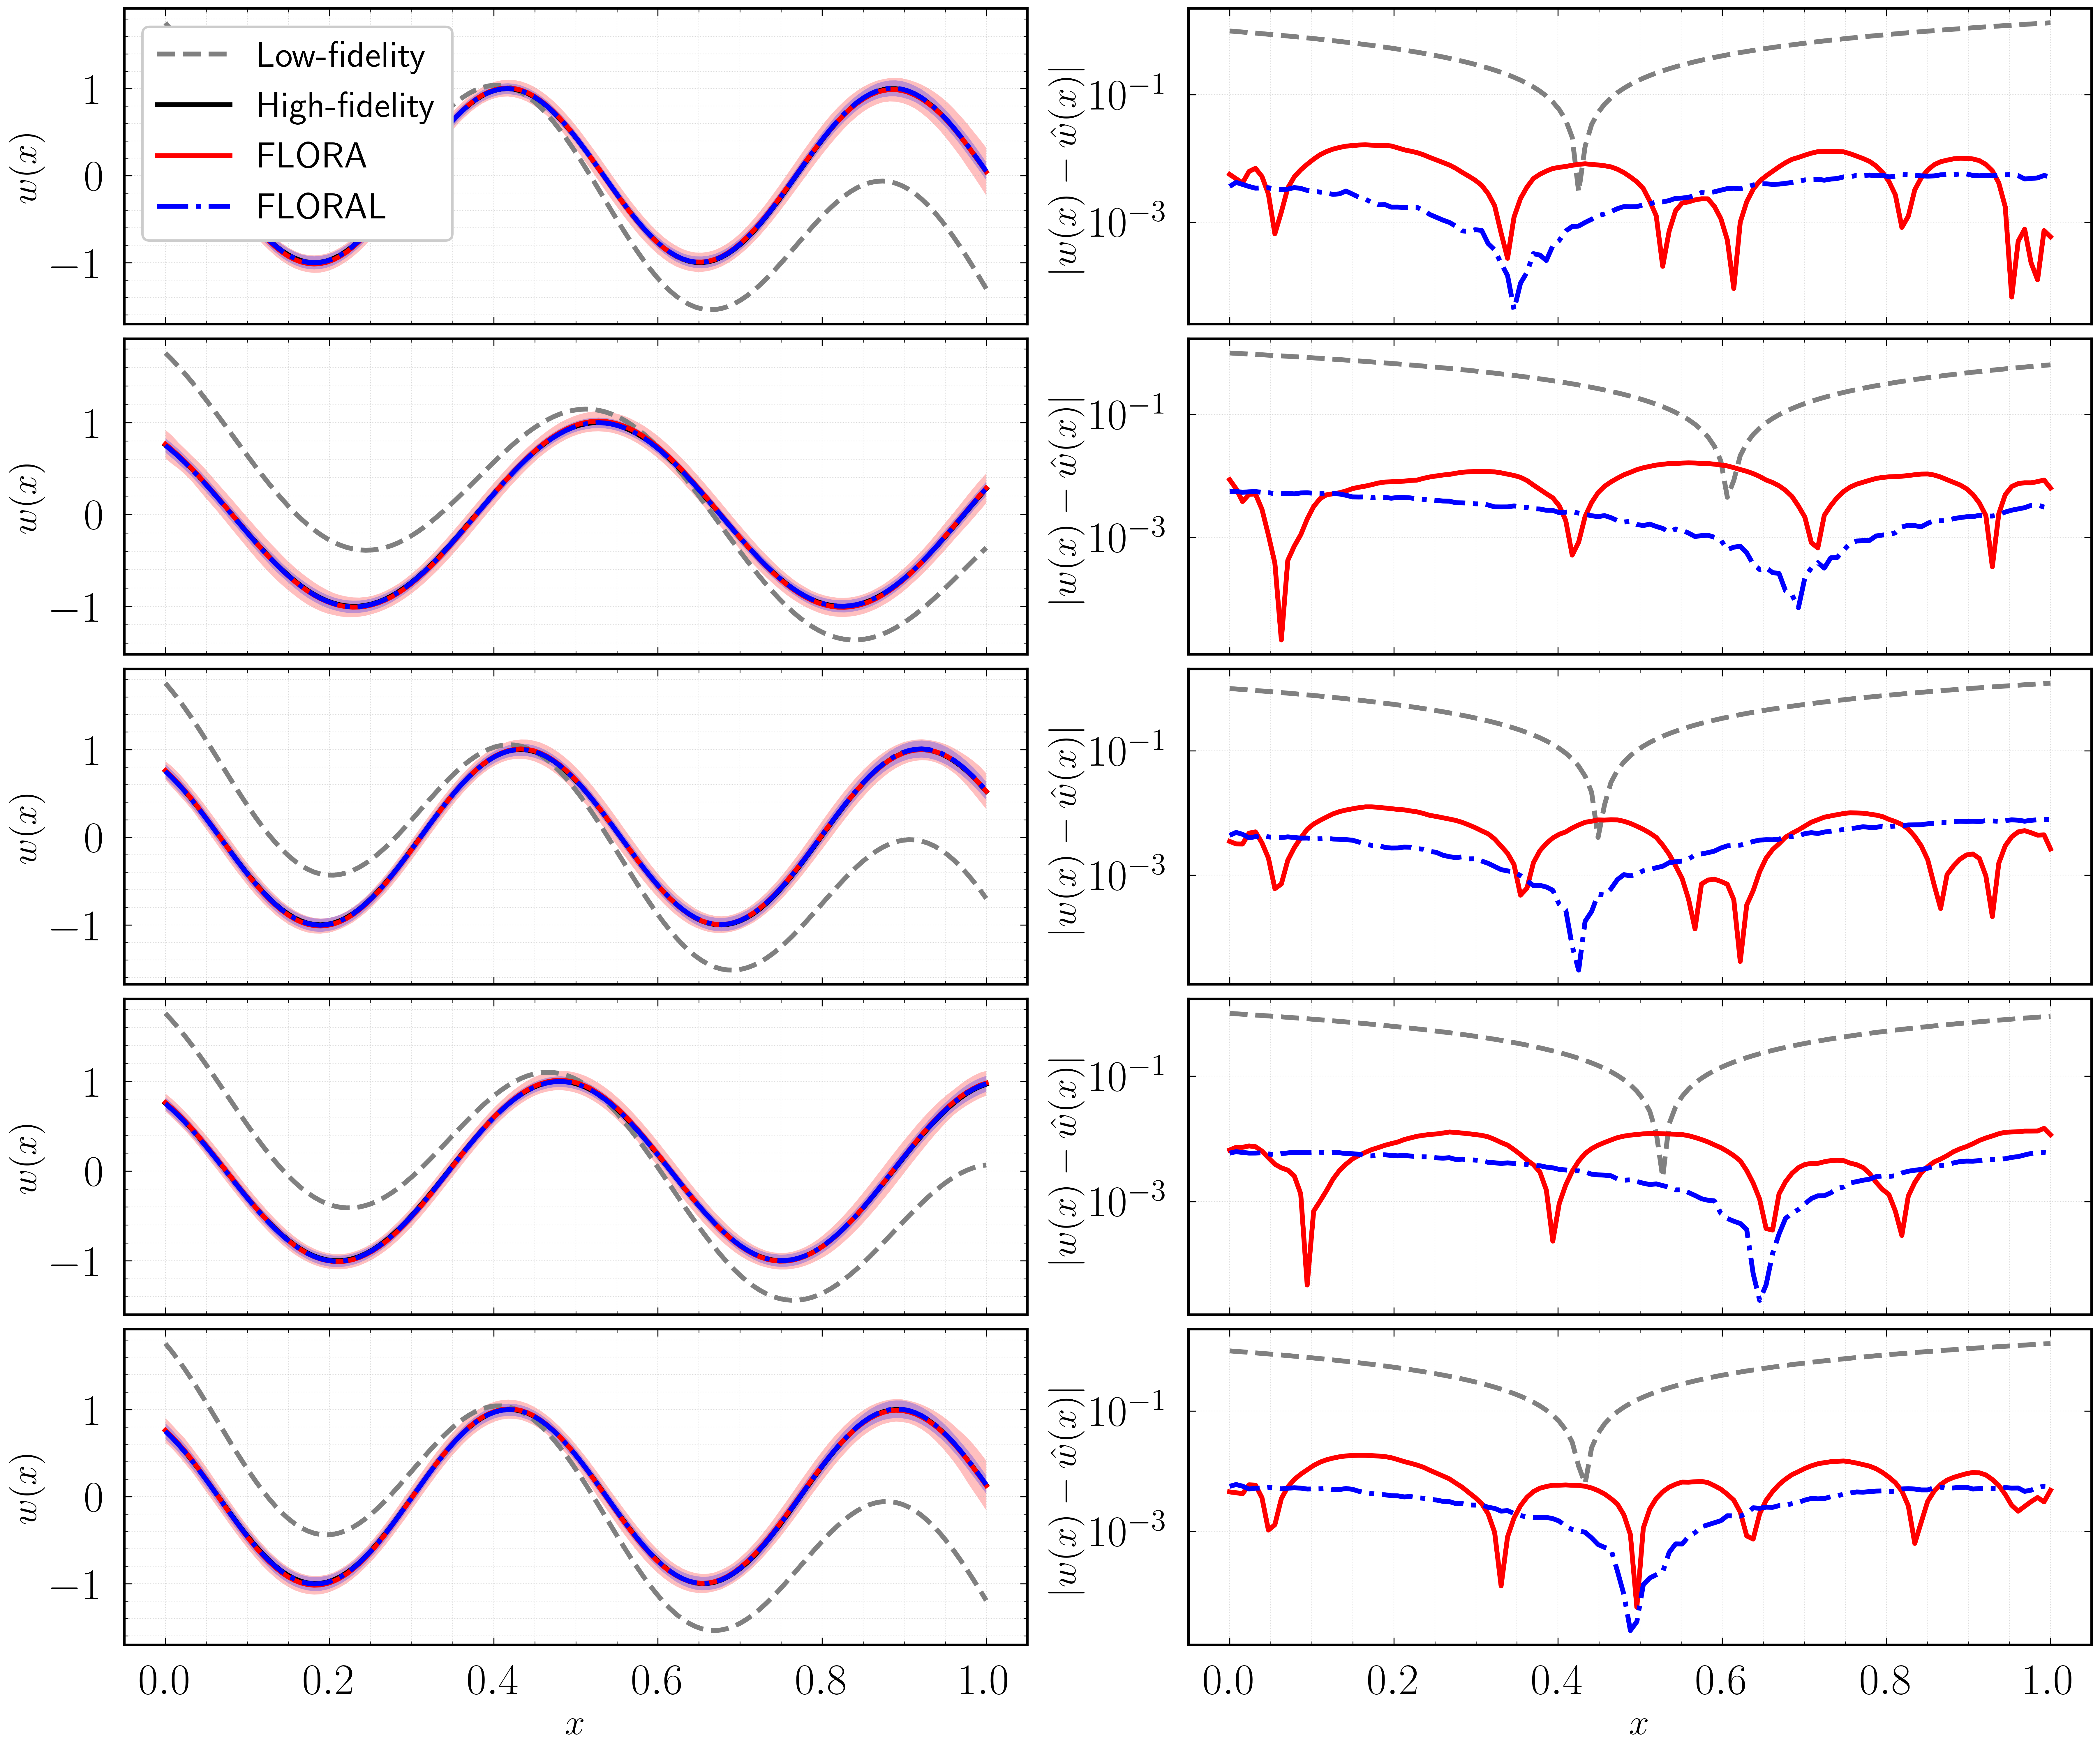}
    \caption{Samples of the generated high-fidelity function (left) using \textsc{flora} (\textcolor{red}{\fline}) and \textsc{floral} (\textcolor{blue}{\dashdot}) and the absolute error (right) for the 1D problem with input function correlation.
    The shaded region indicates $\pm 10$ standard deviations about the mean for both models, computed using $100$ generated ensembles.
    Model trained with $10$ high-fidelity and corresponding low-fidelity training samples for a training and inference resolution of $128$ discretization points.
    Samples are generated on the same input function as in~\cref{fig:onedcorr/samples_10_train_full_res}.}
    \label{fig:ondcorr/appendix/samples_1000_train_full_res}
\end{figure}
\Cref{fig:ondcorr/appendix/samples_1000_train_full_res} illustrates samples of the generated high-fidelity function using \textsc{flora} and \textsc{floral} along with the absolute error when trained with $1000$ high-fidelity training samples.
Here, the low-fidelity and high-fidelity training and inference resolutions are all set to $128$ discretization points.
\Cref{fig:onedcorr/appendix/error_comparison} compares the RMSE, NRMSE, and CRMSE metrics of the proposed multi-fidelity probabilistic neural operator framework against single-fidelity baselines.
As shown in~\cref{fig:onedcorr/appendix/samples_superresolution_train_res_64}, even when the model is trained at a reduced resolution of $64$ discretization points and evaluated at $128$ points ($2\times$ resolution increase), the predictive uncertainty is still reduced.
\begin{figure}[h!]
\centering
    \includegraphics[width=1.0\textwidth]{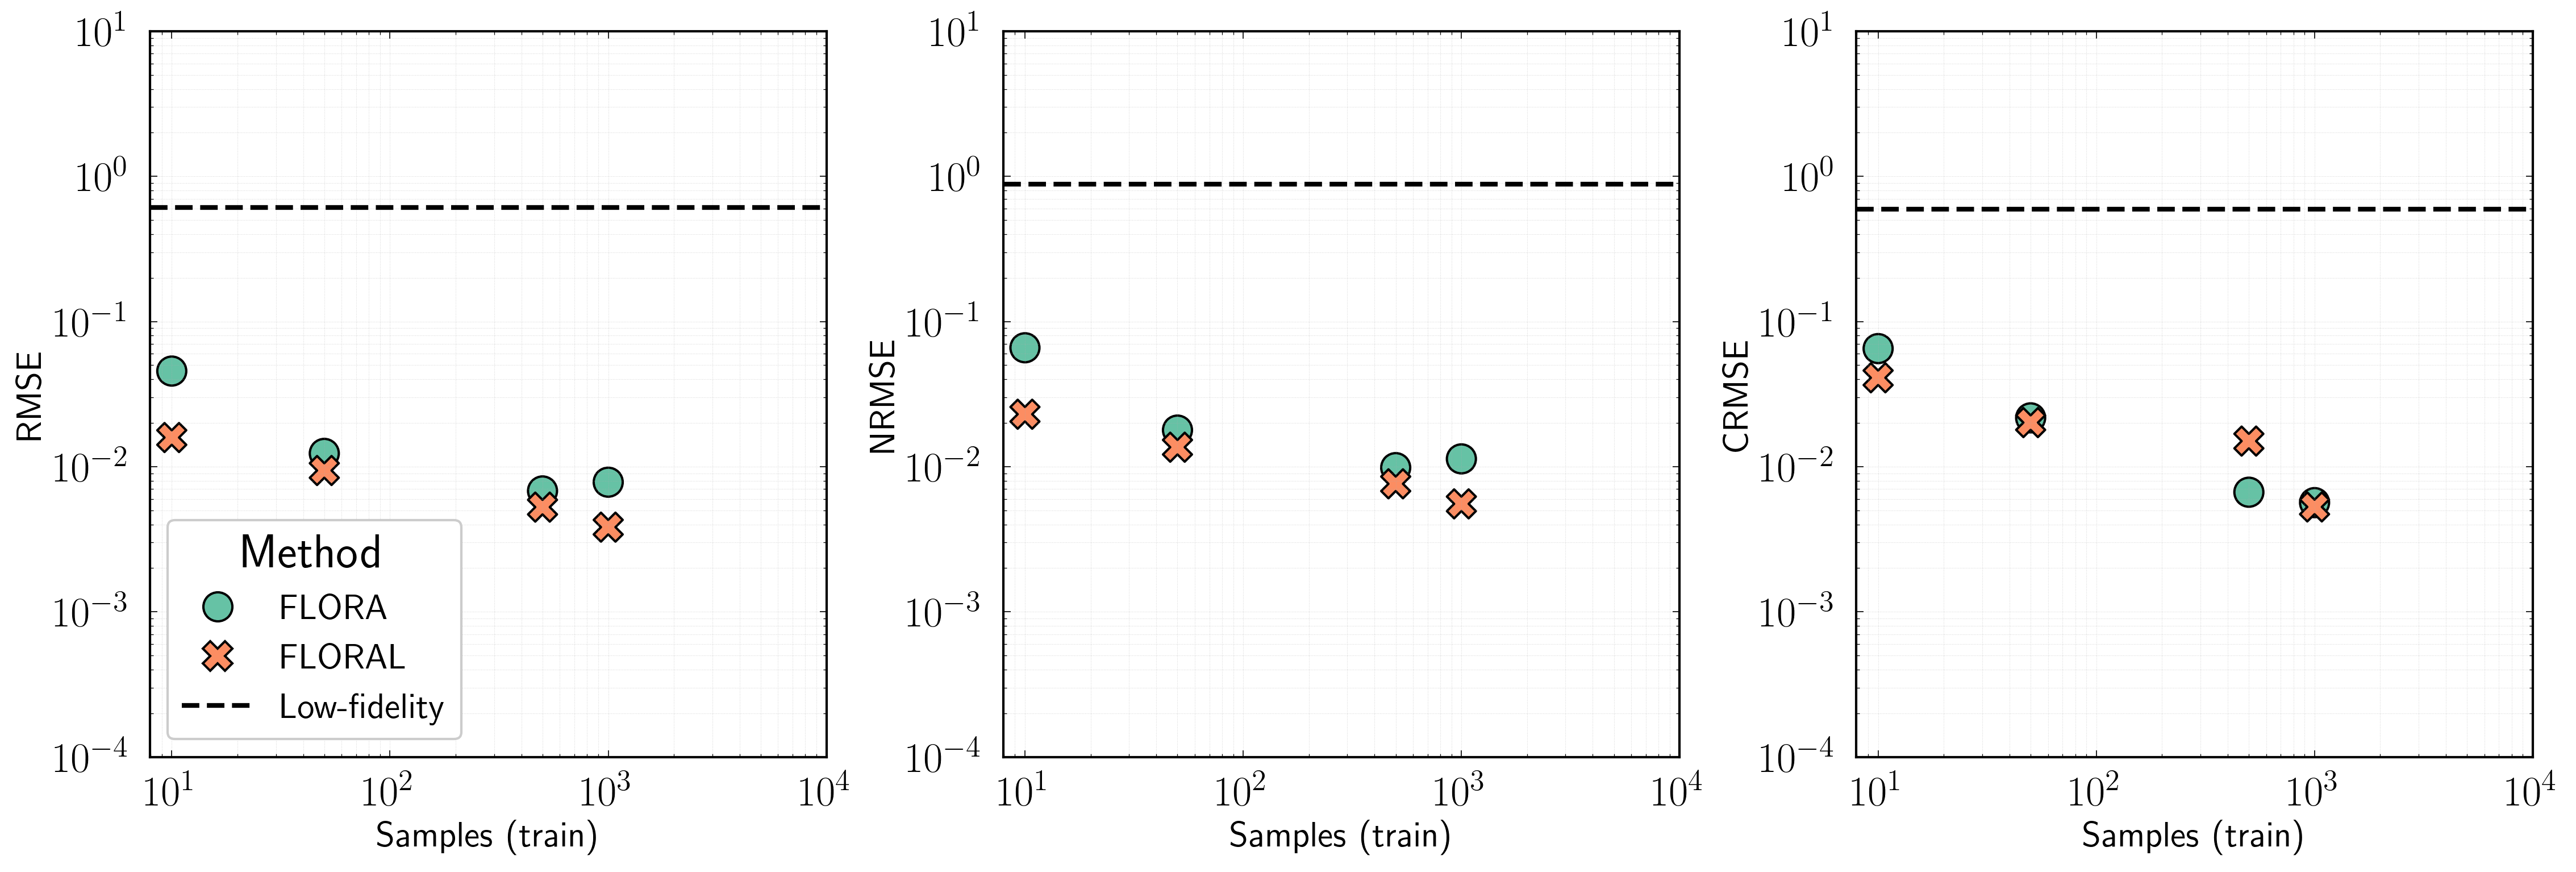}
    \caption{Comparison of RMSE (left), NRMSE (center), and CRMSE (right) for the 1D problem with input function dependent correlation.
    To compute the statistics, $1000$ unseen high-fidelity function samples are used, and for each sample, $100$ ensembles are generated for the probabilistic models.
    Training and inference resolution set to $128$ discretization points.
    }
    \label{fig:onedcorr/appendix/error_comparison}
\end{figure}
\begin{figure}[h!]
    \centering
    \includegraphics[width=0.8\textwidth]{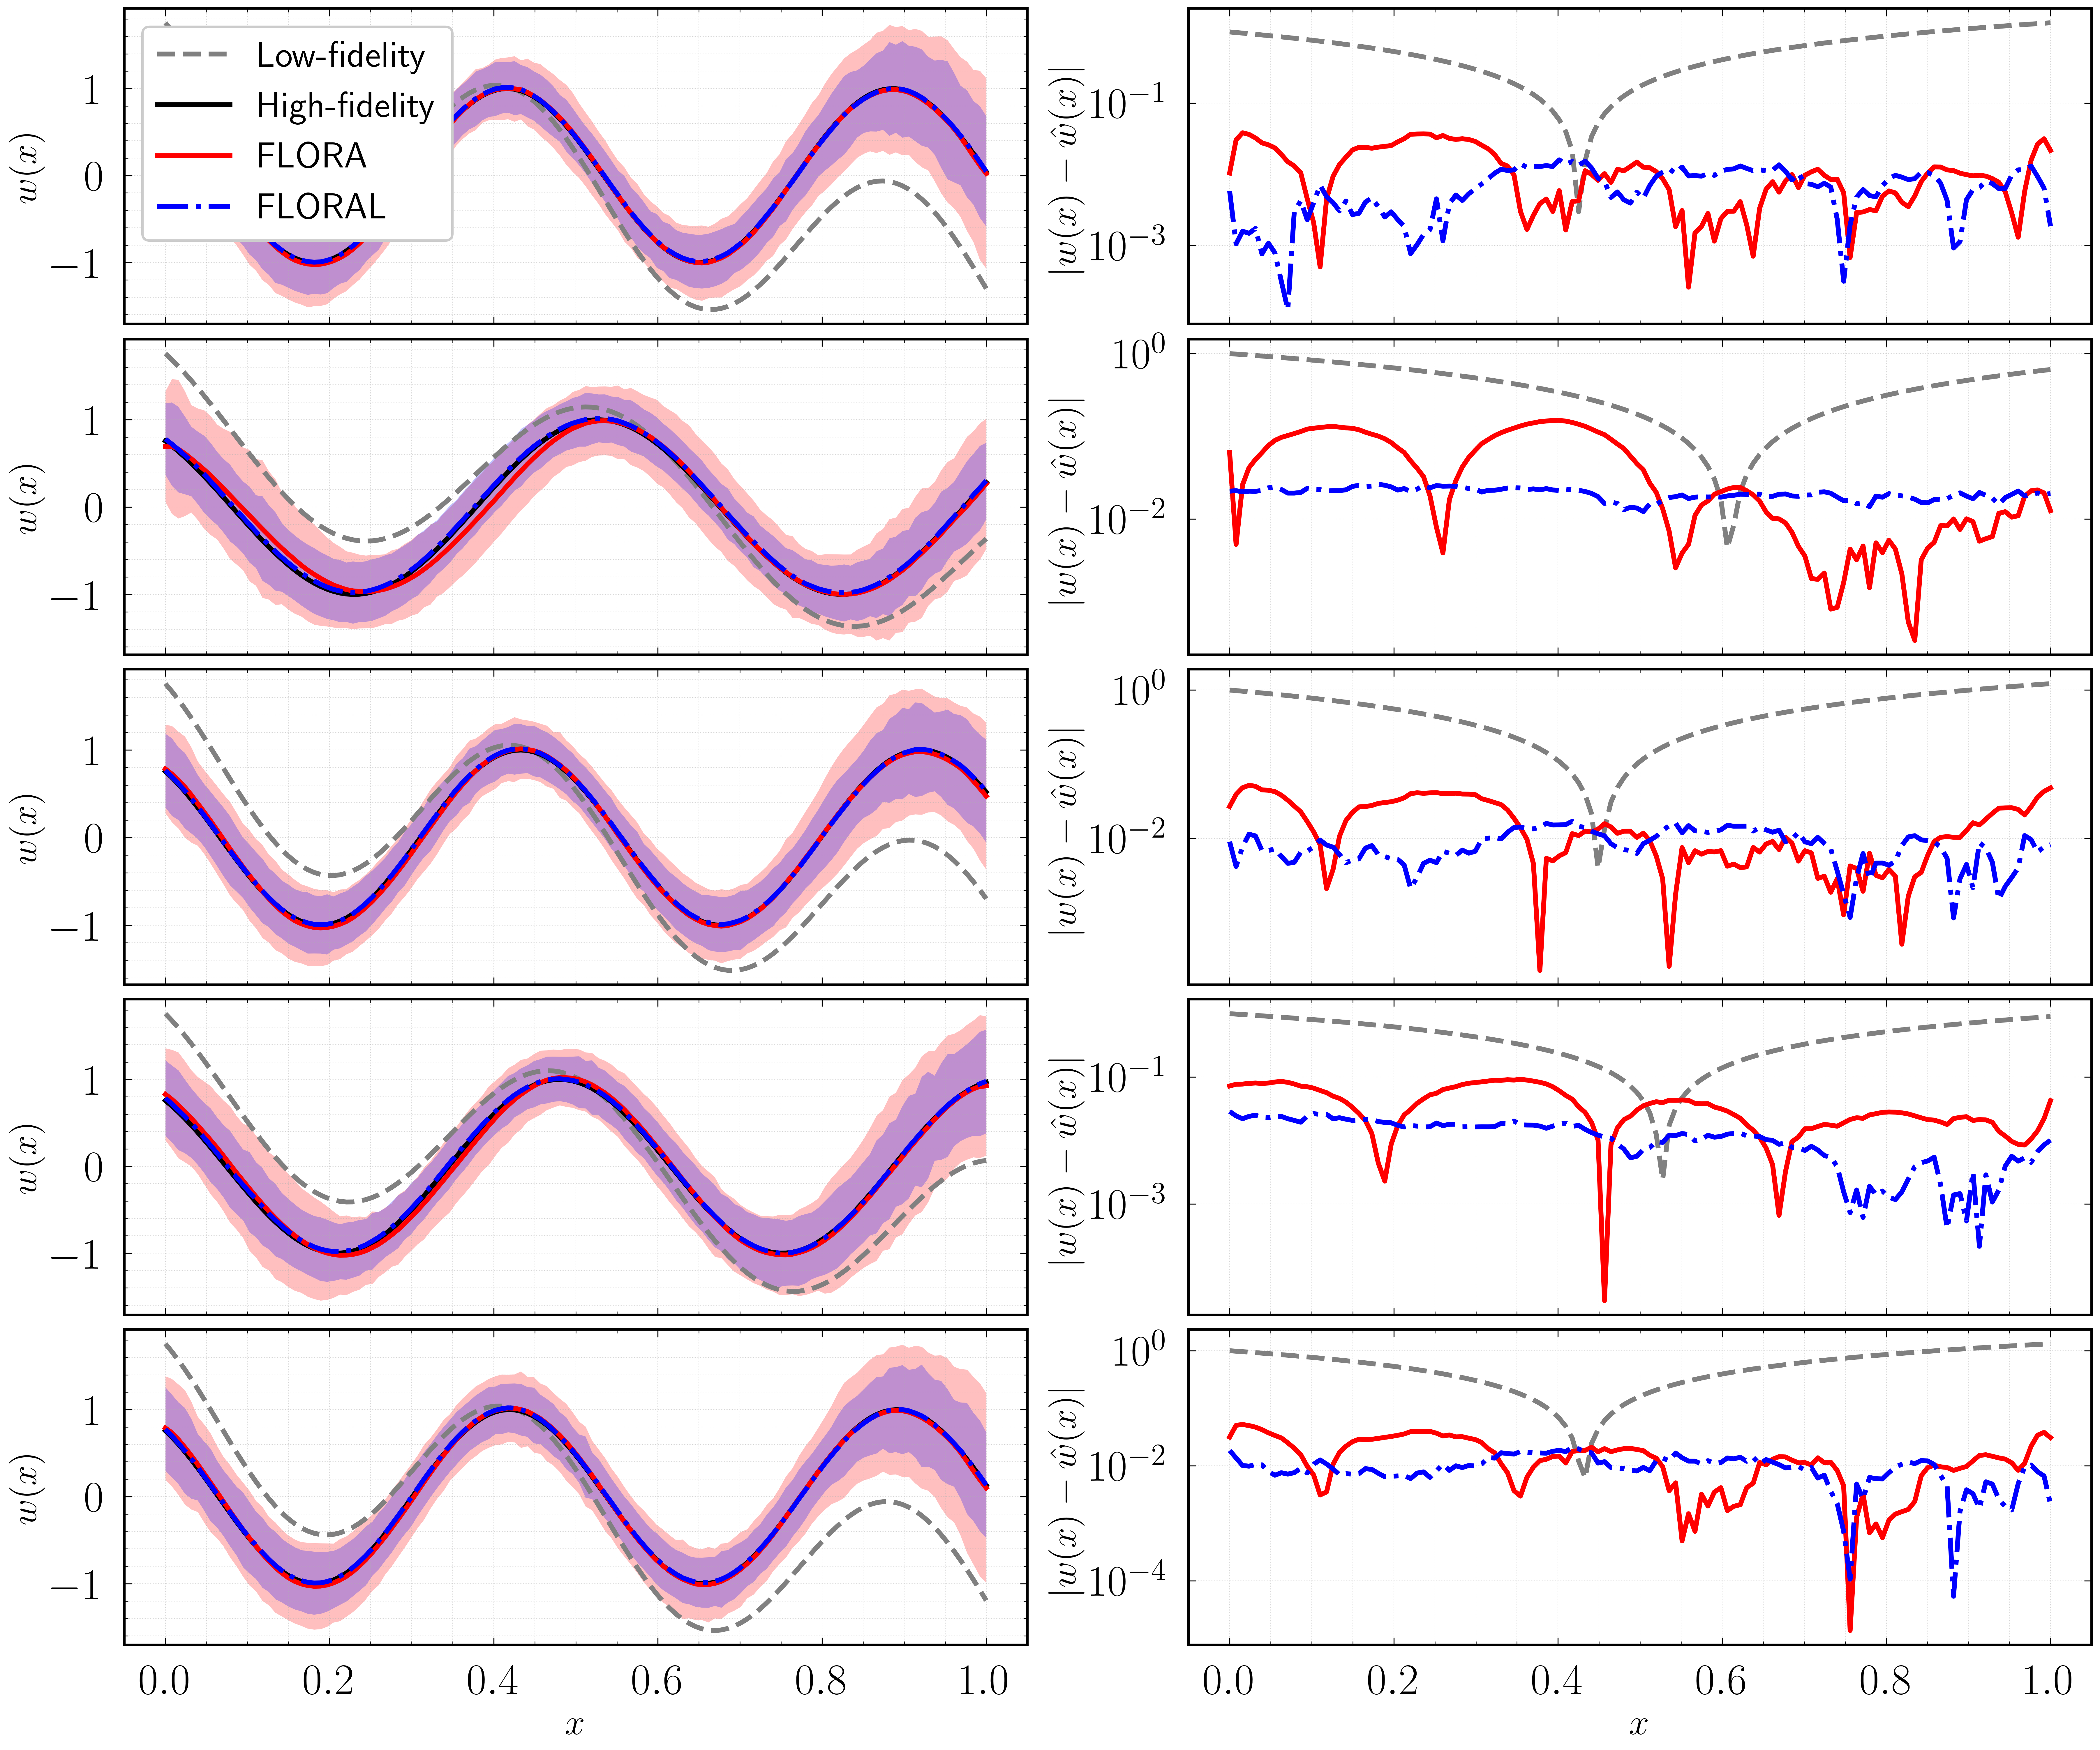}
    \caption{Samples of the generated high-fidelity function (left) using $\textsc{flora}$ (\textcolor{red}{\fline}) and $\textsc{floral}$ (\textcolor{blue}{\dashdot}) and the absolute error (right) for the 1D problem with input function correlation.
    The shaded region indicates $\pm 10$ standard deviations about the mean for both models, computed using $100$ generated ensembles.
    Model trained with $10$ high-fidelity training samples using $64$ discretization points, and inference is performed on $128$ points, that is, a $2\times$ resolution increase.
    Samples are generated on the same input function as in~\cref{fig:onedcorr/samples_10_train_full_res}.}
    \label{fig:onedcorr/appendix/samples_superresolution_train_res_64}
\end{figure}

%% <<< AP1

%% >>> Advection
\subsection{1D advection equation}\label{sec:appendix/advection}
\begin{table}[h!]
\centering
    \caption{Training configurations for the 1D advection equation. The training and inference resolutions are common across spatial and temporal resolutions.
    The number of Fourier modes is common to both spatial and temporal dimensions.
    }
\label{tab:advection/config}
\begin{tabular}{cccccc}
\toprule
\makecell{\textbf{Train$\to$Infer}\\\textbf{Resolution}} &
\textbf{Epochs} &
\makecell{\textbf{Train}\\\textbf{Size}} &
\makecell{\textbf{Validation}\\\textbf{Size}} &
\makecell{\textbf{Batch}\\\textbf{Size}} &
\makecell{\textbf{\# Fourier}\\\textbf{Modes}} \\
\midrule
\multirow{3}{*}{128 $\to$ 128}
    & \multirow{3}{*}{500} & 500      & \multirow{3}{*}{1{,}000} & 16   & \multirow{3}{*}{64} \\
    & & 1{,}000      &  & 64   & \\
    & & 5{,}000     & & 128  & \\
\bottomrule
\end{tabular}
\end{table}
For training the models, the configurations are tabulated in~\cref{tab:advection/config}.
\Cref{fig:advection/appendix/samples_5000_train} illustrates the absolute error in the solution obtained using the low-fidelity model, \textsc{flora}, and \textsc{floral} on unseen initial conditions when trained with $5000$ high-fidelity training samples.
We use the same initial conditions as in~\cref{fig:advection/samples_500_train_full_res}, and, as shown, increasing the number of high-fidelity training samples improves predictive accuracy and reduces predictive uncertainty for both models.

\begin{figure}[h!]
    \centering
    \includegraphics[width=0.55\textwidth]{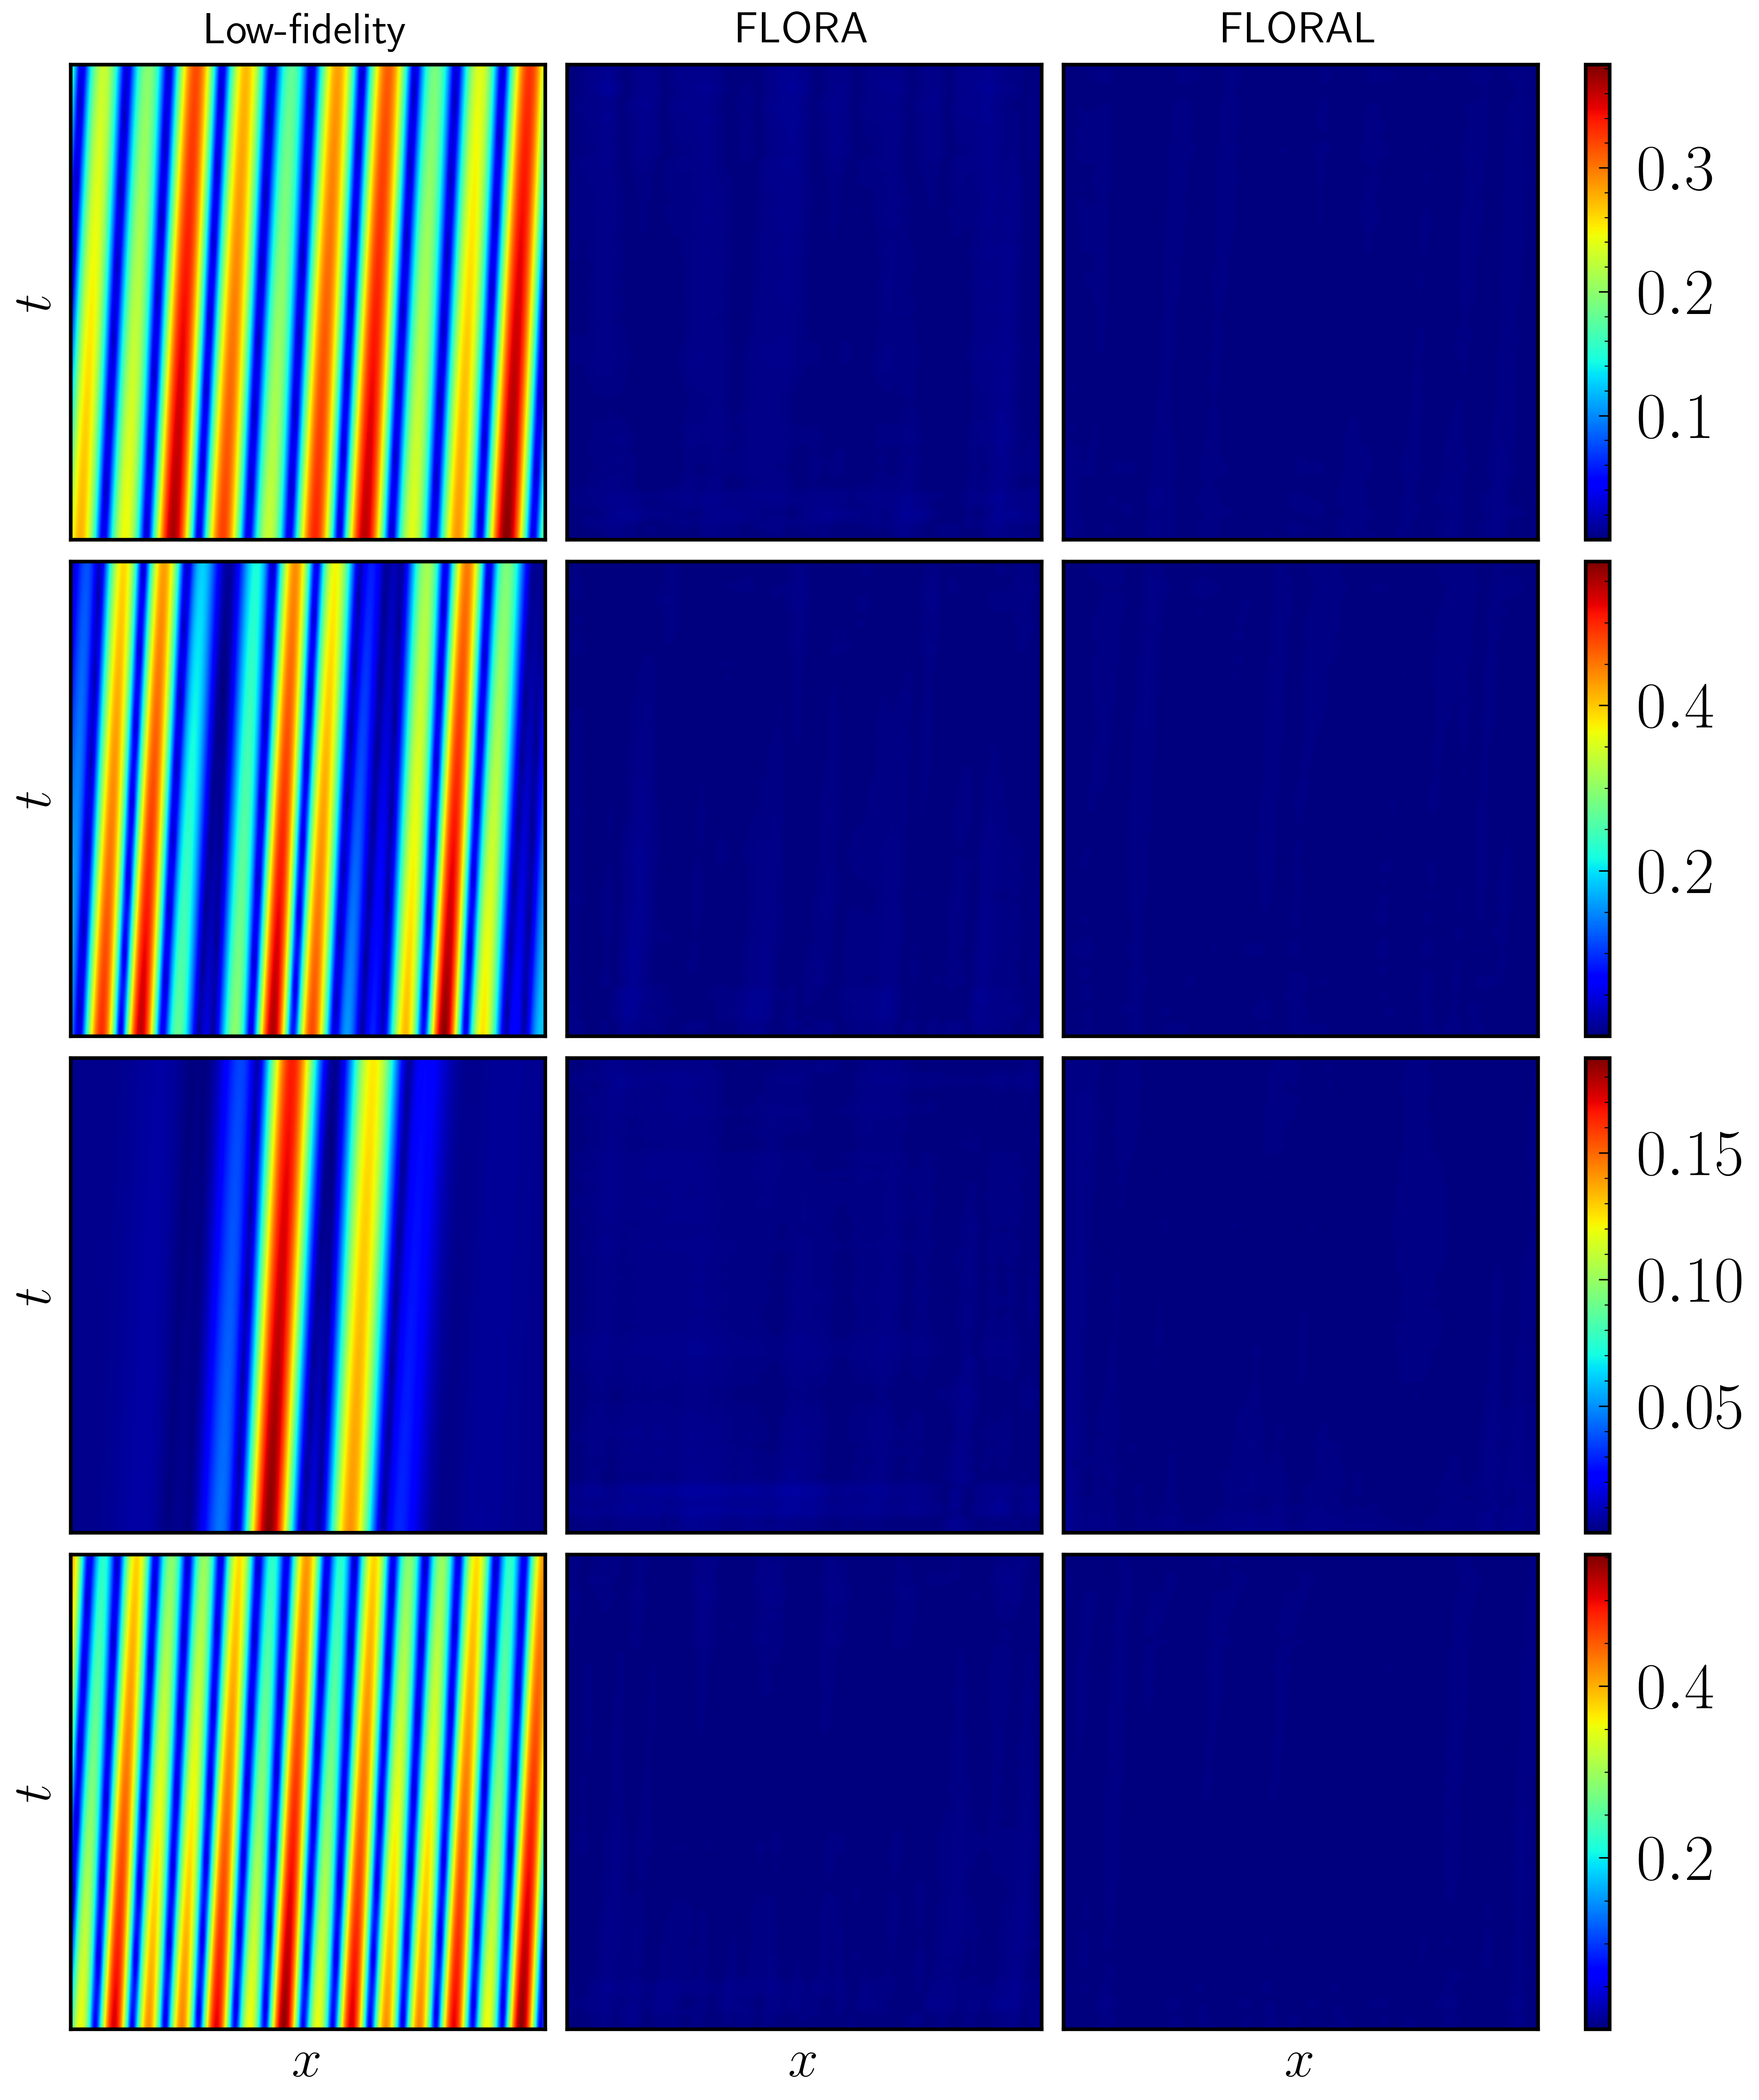}
    \caption{Illustration of absolute error in the solution obtained using low-fidelity model (left), \textsc{flora} (center), and \textsc{floral} (right) on unseen initial conditions for the 1D advection equation.
    Model trained with $5000$ high-fidelity and corresponding low-fidelity training samples.
    To compute the mean prediction for probabilistic models, $50$ ensembles are generated for each unseen initial condition.
    Samples are generated on the same initial conditions as in~\cref{fig:advection/samples_500_train_full_res}.}
    \label{fig:advection/appendix/samples_5000_train}
\end{figure}

%% <<< Advection

%% >>> Burgers
\subsection{1D Burgers' equation}\label{sec:appendix/burgers}
\begin{table}[h!]
\centering
    \caption{Training configurations for the 1D Burgers' equation. The training and inference resolutions are common across spatial and temporal resolutions.
    The number of Fourier modes is common to both spatial and temporal dimensions.
    }
\label{tab:burgers/config}
\begin{tabular}{cccccc}
\toprule
\makecell{\textbf{Train$\to$Infer}\\\textbf{Resolution}} &
\textbf{Epochs} &
\makecell{\textbf{Train}\\\textbf{Size}} &
\makecell{\textbf{Validation}\\\textbf{Size}} &
\makecell{\textbf{Batch}\\\textbf{Size}} &
\makecell{\textbf{\# Fourier}\\\textbf{Modes}} \\
\midrule
\multirow{3}{*}{128 $\to$ 128}
    & \multirow{3}{*}{500} & 500      & \multirow{3}{*}{1{,}000} & 16   & \multirow{3}{*}{64} \\
    & & 1{,}000      &  & 64   & \\
    & & 5{,}000     & & 128  & \\
\bottomrule
\end{tabular}
\end{table}

For training the models, the configurations are tabulated in~\cref{tab:burgers/config}.
\Cref{fig:burgers/appendix/samples_5000_train} illustrates the absolute error in the solution obtained using the low-fidelity model, \textsc{flora}, and \textsc{floral} on unseen initial conditions when trained with $5000$ high-fidelity training samples.
We use the same initial conditions as in~\cref{fig:burgers/samples_500_train_full_res}, and, as shown, increasing the number of high-fidelity training samples improves predictive accuracy and reduces predictive uncertainty for both models.

\begin{figure}[h!]
    \centering
    \includegraphics[width=0.55\textwidth]{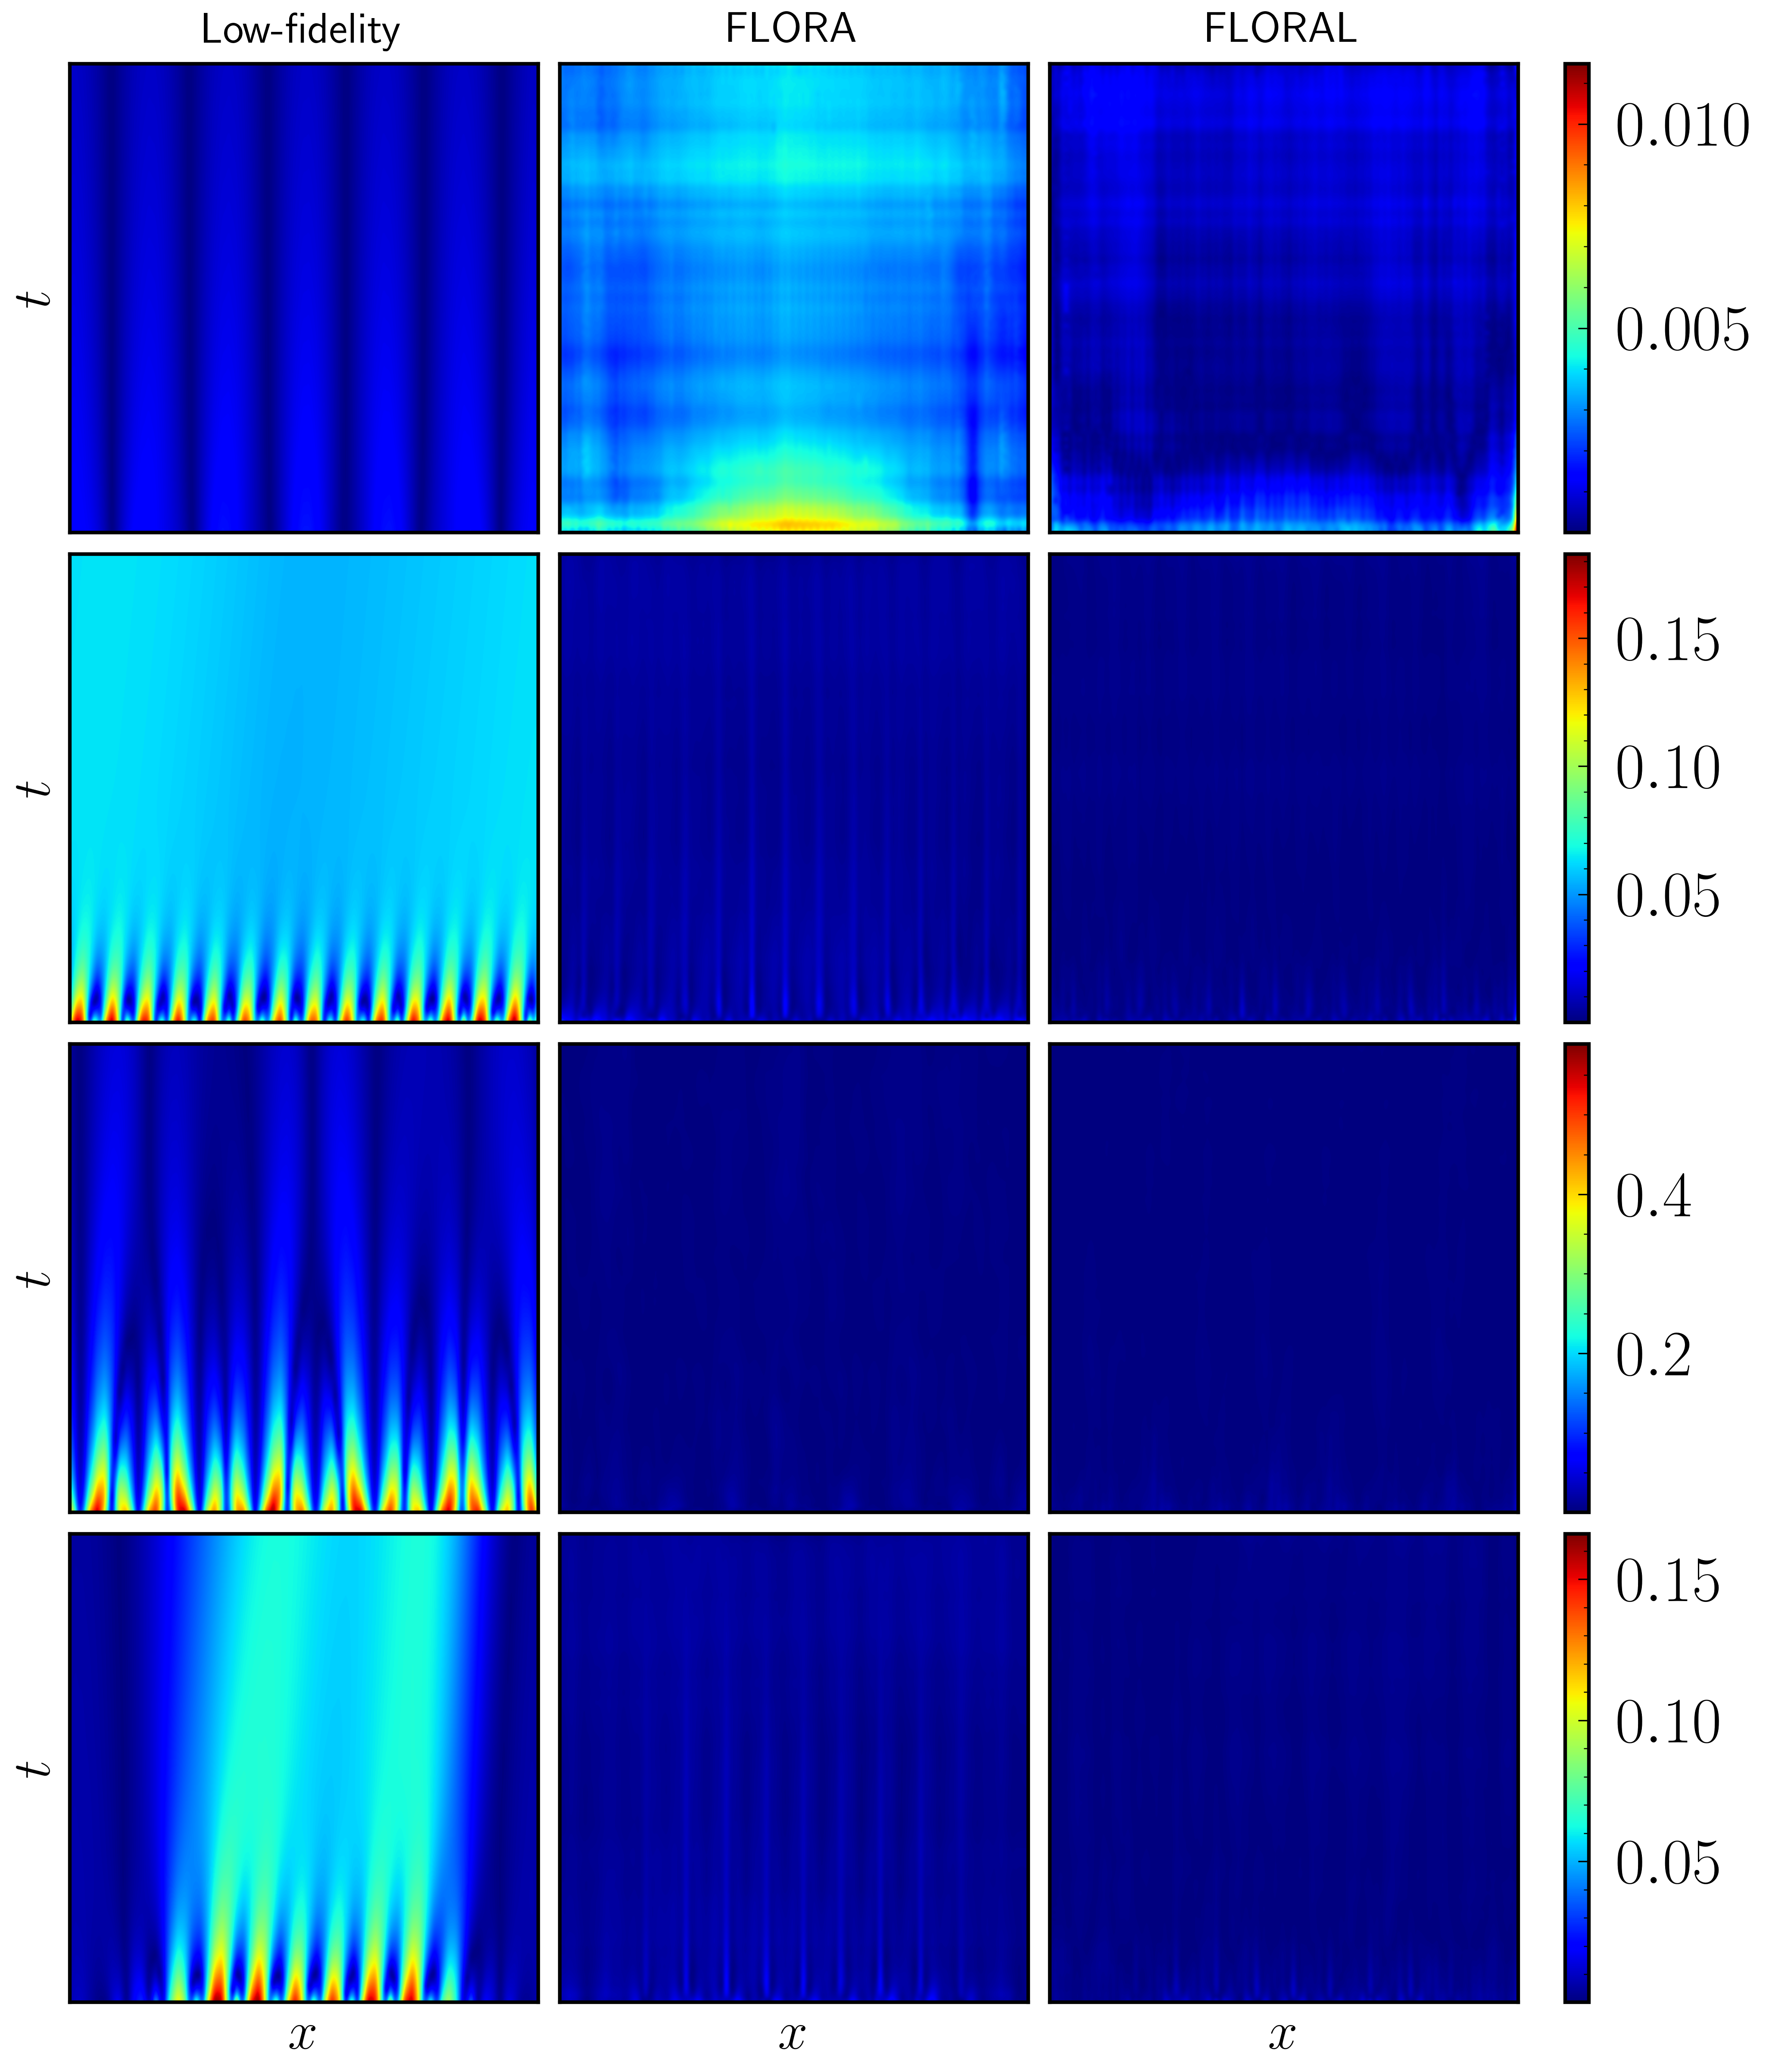}
    \caption{Illustration of absolute error in the solution obtained using low-fidelity model (left), \textsc{flora} (center), and \textsc{floral} (right) on unseen initial conditions for the 1D Burgers' equation.
    Model trained with $5000$ high-fidelity training samples and corresponding low-fidelity training samples.
    To compute the mean prediction for probabilistic models, $50$ ensembles are generated for each unseen initial condition.
    Samples are generated on the same initial conditions as in~\cref{fig:burgers/samples_500_train_full_res}.}
    \label{fig:burgers/appendix/samples_5000_train}
\end{figure}

%% <<< Burgers

%% >>> Darcy
\subsection{Darcy flow}\label{sec:appendix/darcy}
\begin{table}[h!]
\centering
    \caption{Training configurations for the Darcy flow. The training and inference resolutions are common across spatial and temporal resolutions.
    The number of Fourier modes is common to both spatial and temporal dimensions.
    }
\label{tab:darcy/config}
\begin{tabular}{cccccc}
\toprule
\makecell{\textbf{Train$\to$Infer}\\\textbf{Resolution}} &
\textbf{Epochs} &
\makecell{\textbf{Train}\\\textbf{Size}} &
\makecell{\textbf{Validation}\\\textbf{Size}} &
\makecell{\textbf{Batch}\\\textbf{Size}} &
\makecell{\textbf{\# Fourier}\\\textbf{Modes}} \\
\midrule
\multirow{3}{*}{128 $\to$ 128}
    & \multirow{3}{*}{500} & 500      & \multirow{3}{*}{1{,}000} & 16   & \multirow{3}{*}{64} \\
    & & 1{,}000      &  & 64   & \\
    & & 5{,}000     & & 128  & \\
\bottomrule
\end{tabular}
\end{table}
For training the models, the configurations are tabulated in~\cref{tab:darcy/config}.
\Cref{fig:darcy/appendix/samples_5000_train_full_res} illustrates the absolute error in the solution obtained using the low-fidelity model, \textsc{flora}, and \textsc{floral} on unseen permeability fields when trained with $5000$ high-fidelity training samples.
We use the same permeability fields as in~\cref{fig:darcy/samples_500_train_full_res}, and, as shown, increasing the number of high-fidelity training samples improves predictive accuracy and reduces predictive uncertainty for both models.

\begin{figure}[h!]
    \centering
    \includegraphics[width=0.55\textwidth]{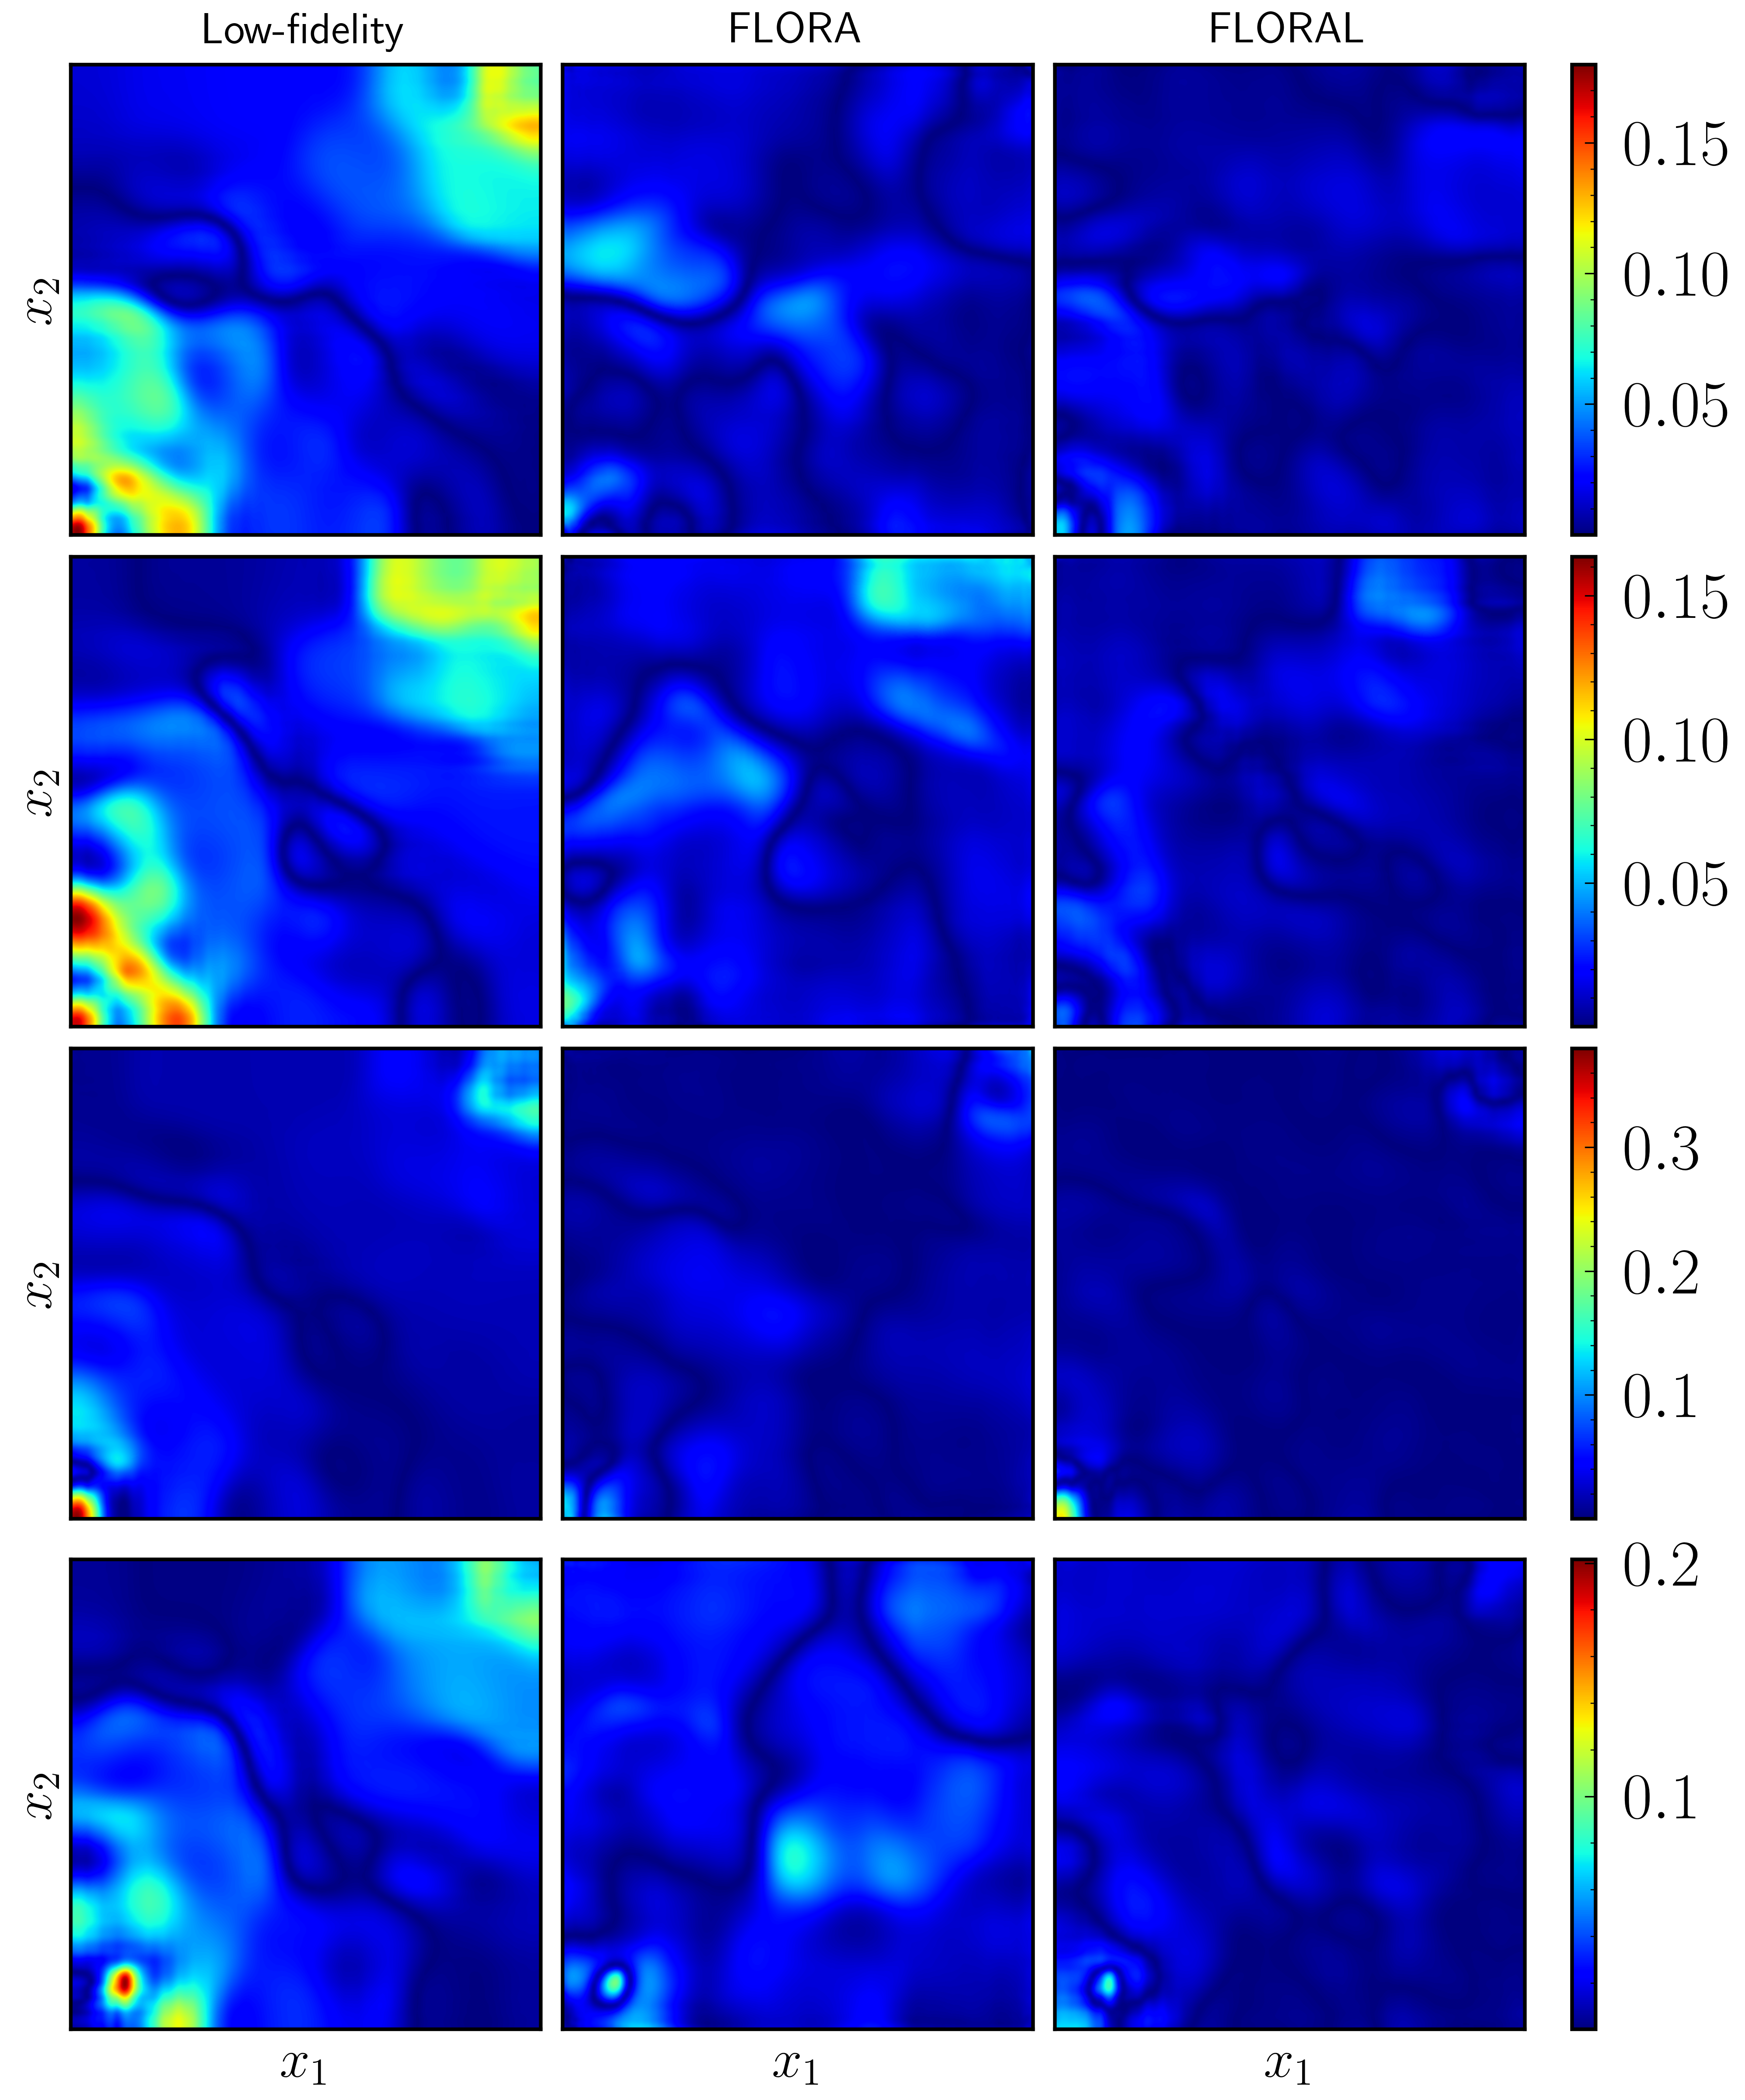}
    \caption{Illustration of absolute error in the solution obtained using low-fidelity model (left), \textsc{flora} (center), and \textsc{floral} (right) on unseen permeability fields for the Darcy flow.
    Model trained with $5000$ high-fidelity training samples and corresponding low-fidelity training samples.
    To compute the mean prediction for probabilistic models, $50$ ensembles are generated for each permeability field.
    Samples are generated on the same permeability fields conditions as in~\cref{fig:darcy/samples_500_train_full_res}.}
    \label{fig:darcy/appendix/samples_5000_train_full_res}
\end{figure}

%% <<< Darcy
